# Supplementary material for: Optimal Control of Material Micro-Structures
Source: arXiv:2210.06734 source file (2022-10-13)
Supplement: Supplementary file 1 [file Appendix.tex]

\newpage

\section*{Appendix}

\subsection{Iterative Linear Quadratic Regulator Details}

We present details of the D2C-ILQR algorithm in the following. The 'forward pass' and `backward pass' algorithms are summarized in Algorithms \ref{model_free_DDP_OL_FP} and \ref{model_free_DDP_OL_BP} respectively. Algorithm \ref{model_free_DDP_feedback} presents the DDP feedback algorithm used to calculate the optimal feedback gain. 

\begin{algorithm}
\footnotesize
 \caption{\strut Forward Pass}
  {\bf Input:} Nominal trajectory - $\mathbb{T}_{nom}^{k}$, previous iteration policy parameters - $\{k_{0:N-1}, K_{0:N-1}\}$ and system and cost parameters - $\mathcal{P}$.\
%   \CommentSty{/* Unpack the previous nominal trajectory.*/}\\
  $\{{\bar{x}_t^{prev}, \bar{u}_t^{prev}}\} \gets \mathbb{T}_{nom}^{k}$.\\
%   \CommentSty{/* Initialize time to 0.*/}\\
  $t \gets 0$.\\
  \While {$t < N$}{
    %\CommentSty{/*$\alpha$ is the line-search parameter.*/} \\
    \CommentSty{/*Simulate one step forward ($\alpha$ is the line-search parameter.)*/}
    \begin{equation*}
    \begin{split}
        {\bar{u}_{t}} &= {\bar{u}_t^{prev}} + \alpha k_t + K_{t} ({\bar{x}_t} - {\bar{x}_t^{prev}}),\\
        {\bar{x}_{t+1}} &= simulate\_forward\_step({\bar{x}_t}, {\bar{u}_t}).
        \end{split}
    \end{equation*}
    $t \leftarrow t + 1$. 
    }
  $\mathbb{T}_{nom}^{k+1}$ $\gets$ $\{{\bf \bar{x}_{0:N}}, {\bf \bar{u}_{0:N-1}}\}.$\\
  \If{$\mathbb{T}_{nom}^{k+1}$ to $\mathbb{T}_{nom}^{k}$ \textnormal{is acceptable}}{
    {\bf return} $\mathbb{T}_{nom}^{k+1}$, true.
  }
  \Else{
    {\bf return} $\mathbb{T}_{nom}^{k}$, false.
  }
  \label{model_free_DDP_OL_FP}
\end{algorithm}
\begin{algorithm} 
\footnotesize
  \caption{\strut Backward Pass}
  {\bf Input:} Nominal trajectory - $\mathbb{T}_{nom}^{k}$, previous iteration policy parameters - $\{k_{0:N-1}, K_{0:N-1}\}$, horizon - N and system and cost parameters - $\mathcal{P}$.\\
  \CommentSty{/* Backward pass starts from the final time-step i.e, N-1.*/}\\
  $t \gets N - 1$.\ \\
  Compute $J_{x_N}$ and $J_{x_N x_N}$ using boundary conditions.\\
  \CommentSty{/*Keep a copy of previous policy gains.*/}\\
  $k\_old \gets k_{0:N}$ {and}  $K\_old \gets K_{0:N}$.\\
  
  \While {$t >= 0$}{
  \CommentSty{/*Obtain the Jacobians from simulator rollouts as shown in Section \ref{sys_id_solve}:*/}\\
  $f_{x_t}, f_{u_t} \gets model\_free\_jacobian({ \bar{x}_t},{\bar{u}_t}).$\\
  \CommentSty{/*Obtain the partials of the Q function as follows:*/}
    \begin{equation*}
    \begin{split}
    Q_{x_t} &= c_{x_t}  + h_{x_t}^T J_{x_{t+1}}^{\prime},\\
    Q_{u_t} &= c_{u_t} + h_{u_t}^T J_{x_{t+1}}^{\prime},\\
    Q_{x_t x_t} &= c_{x_t x_t} + h_{x_t}^T J_{x_{t+1} x_{t+1}}^{\prime} h_{x_t}, \\
    Q_{u_t x_t} &= c_{u_t x_t} + h_{u_t}^T (J_{x_{t+1} x_{t+1}}^{\prime} + \mu I_{n_x \times n_x}) h_{x_t}, \\
    Q_{u_t u_t} &= c_{u_t u_t} + h_{u_t}^T (J_{x_{t+1} x_{t+1}}^{\prime} + \mu I_{n_x \times n_x}) h_{u_t}.\\
    \end{split}
\end{equation*}
  \If{$Q_{u_t u_t}$ {\textnormal{is positive-definite}}}{
    \begin{equation*}
    \begin{split}
        k_t &= -Q_{u_t u_t}^{-1} Q_{u_t},\\
        K_t &= -Q_{u_t u_t}^{-1} Q_{u_t x_t}.
        \end{split}
    \end{equation*}
    }
    
%   \Endif
  \Else{
    \CommentSty{/*If $Q_{u_t u_t}$ is not positive-definite, then, abort the backward pass.*/}\\
    {\bf return } $\{ k\_old, K\_old\}$, false.
  }
  \CommentSty{/*Obtain the partials of the value function $J_t$ as follows:*/}
  \begin{equation*}
      \begin{split}
          J_{x_t} &= Q_{x_t} + K_{t}^T Q_{u_t u_t} k_t + K_t^T Q_{u_t} + Q_{u_t x_t}^T k_t,\\
          J_{x_t x_t} &= Q_{x_t x_t} + K_t^T Q_{u_t u_t} K_t + K_t^T Q_{u_t x_t} + Q_{u_t x_t}^T K_t.
      \end{split}
  \end{equation*}
  $t \leftarrow t - 1$ 
  }
  $k\_new = k_{0:N-1},$\\
  $K\_new = K_{0:N-1}.$\\
  {\bf return} $\{k\_new, K\_new\}$, true.
  \label{model_free_DDP_OL_BP}
\end{algorithm}

\begin{algorithm} 
\footnotesize
  \caption{\strut DDP Feedback}
  {\bf Input:} Nominal trajectory - $\mathbb{T}_{nom}^{k}$, horizon - N and system and cost parameters - $\mathcal{P}$.\\
  \CommentSty{/* Start from the final time-step i.e, N-1.*/}\\
  $t \gets N - 1$.\ \\
  Compute $J_{x_N}$ and $J_{x_N x_N}$ using boundary conditions.\\

  \While {$t >= 0$}{
  \CommentSty{/*Obtain the Jacobians from simulator rollouts as shown in Section \ref{sys_id_solve}:*/}\\
  $h_{x_t}, h_{u_t} \gets model\_free\_jacobian({ \bar{x}_t},{\bar{u}_t}).$\\
  \CommentSty{/*Obtain the Hessians from simulator rollouts as shown above:*/}\\
  $h_{x_tx_t}, h_{u_tx_t}, h_{u_tu_t} \gets model\_free\_hessian({ \bar{x}_t},{\bar{u}_t}).$\\
  \CommentSty{/*Obtain the partials of the Q function as follows:*/}
    \begin{equation*}
    \begin{split}
    Q_{x_t} &= c_{x_t}  + h_{x_t}^T J_{x_{t+1}}^{\prime},\\
    Q_{u_t} &= c_{u_t} + h_{u_t}^T J_{x_{t+1}}^{\prime},\\
    Q_{x_t x_t} &= c_{x_t x_t} + h_{x_t}^T J_{x_{t+1} x_{t+1}}^{\prime} h_{x_t} + J_{x_{t+1}}^{\prime}h_{x_tx_t}, \\
    Q_{u_t x_t} &= c_{u_t x_t} + h_{u_t}^T (J_{x_{t+1} x_{t+1}}^{\prime} + \mu I_{n_x \times n_x}) h_{x_t} + J_{x_{t+1}}^{\prime}h_{u_tx_t}, \\
    Q_{u_t u_t} &= c_{u_t u_t} + h_{u_t}^T (J_{x_{t+1} x_{t+1}}^{\prime} + \mu I_{n_x \times n_x}) h_{u_t} + J_{x_{t+1}}^{\prime}h_{u_tu_t}.\\
    \end{split}
\end{equation*}
  \If{$Q_{u_t u_t}$ {\textnormal{is positive-definite}}}{
    \begin{equation*}
    \begin{split}
        k_t &= -Q_{u_t u_t}^{-1} Q_{u_t},\\
        K_t &= -Q_{u_t u_t}^{-1} Q_{u_t x_t}.
        \end{split}
    \end{equation*}
    }
    
%   \Endif
  \Else{
    \CommentSty{/*If $Q_{u_t u_t}$ is not positive-definite, then, abort the backward pass.*/}\\
    {\bf return } error.
  }
  \CommentSty{/*Obtain the partials of the value function $J_t$ as follows:*/}
  \begin{equation*}
      \begin{split}
          J_{x_t} &= Q_{x_t} + K_{t}^T Q_{u_t u_t} k_t + K_t^T Q_{u_t} + Q_{u_t x_t}^T k_t,\\
          J_{x_t x_t} &= Q_{x_t x_t} + K_t^T Q_{u_t u_t} K_t + K_t^T Q_{u_t x_t} + Q_{u_t x_t}^T K_t.
      \end{split}
  \end{equation*}
  $t \leftarrow t - 1$ 
  }
  $K = K_{0:N-1}.$\\
  {\bf return} $\{K\}$, true.
  \label{model_free_DDP_feedback}
\end{algorithm}

\subsection*{DDP Feedback Gain Calculation}
Once the optimal nominal trajectory is obtained with ILQR, one DDP back pass is conducted to find the linear optimal feedback gain as shown in Algorithm \ref{model_free_DDP_feedback}. Then the linear feedback is wrapped around the nominal control sequence ($u_t = \bar{u}_t + K_t\delta x_t$),where $\delta x_t$ is the state deviation from the nominal state $\bar{x}_t$.

\subsection{DDPG Algorithm Implementation Details}
\label{sec:ddpg}
% Deep Deterministic Policy Gradient (DDPG) is a policy-gradient based off-policy reinforcement learning algorithm that operates in continuous state and action spaces. It relies on two function approximation networks one each for the actor and the critic. The critic network estimates the $Q(s, a)$ value given the state and the action taken, while the actor network engenders a policy given the current state. Neural networks are employed to represent the networks. 

The off-policy characteristic of the algorithm employs a separate behavioral policy by introducing additive noise to the policy output obtained from the actor network. The critic network minimizes loss based on the temporal-difference (TD) error and the actor network uses the deterministic policy gradient theorem to update its policy gradient as shown below:

Critic update by minimizing the loss: 
\begin{equation*}
    L = \frac{1}{N} \Sigma_{i}(y_i - Q(s_i, a_i| \theta^{Q}))^2
\end{equation*}

Actor policy gradient update:
\begin{equation*}
    \nabla_{\theta^{\mu}} \approx \frac{1}{N} \Sigma_i \nabla_a Q(s,a|\theta^{Q})|_{s=s_i,a=\mu(s_i)} \nabla_{\theta^{\mu}} \mu(s|\theta^{\mu})|_{s_i}
\end{equation*}

The actor and the critic networks consist of two hidden layers with the first layer containing 400 ('{\it relu}' activated) units followed by the second layer containing 300 ('{\it relu}' activated) units. The output layer of the actor network has the number of ('tanh' activated) units equal to that of the number of actions in the action space.  

Target networks one each for the actor and the critic are employed for a gradual update of network parameters, thereby reducing the oscillations and a better training stability. The target networks are updated at $\tau = 0.001$. Experience replay is another technique that improves the stability of training by training the network with a batch of randomized data samples from its experience. We have used a batch size of 32 for the inverted pendulum and the cart pole examples, whereas it is 64 for the rest. Finally, the networks are compiled using Adams' optimizer with a learning rate of 0.001. 

To account for state-space exploration, the behavioral policy consists of an off-policy term arising from a random process. We obtain discrete samples from the Ornstein-Uhlenbeck (OU) process to generate noise as followed in the original DDPG method. The OU process has mean-reverting property and produces temporally correlated noise samples as follows:
\begin{equation*}
    dx_t = \Theta (\mu - x_t)dt + \sigma dW
\end{equation*}
where $\Theta$ indicates how fast the process reverts to mean, $\mu$ is the equilibrium or the mean value and $\sigma$ corresponds to the degree of volatility of the process. $\Theta$ is set to 0.15, $\mu$ to 0 and $\sigma$ is annealed from 0.35 to 0.05 over the training process. 

% \clearpage
\subsection{DDPG Trajectories}
%DDPG TRAJECTORIES
\begin{figure}[!htb]
%\captionsetup{width=1\linewidth}

\begin{multicols}{3}
    % \hspace{3.2cm}
      \subfloat[Initial]{\includegraphics[width=\linewidth]{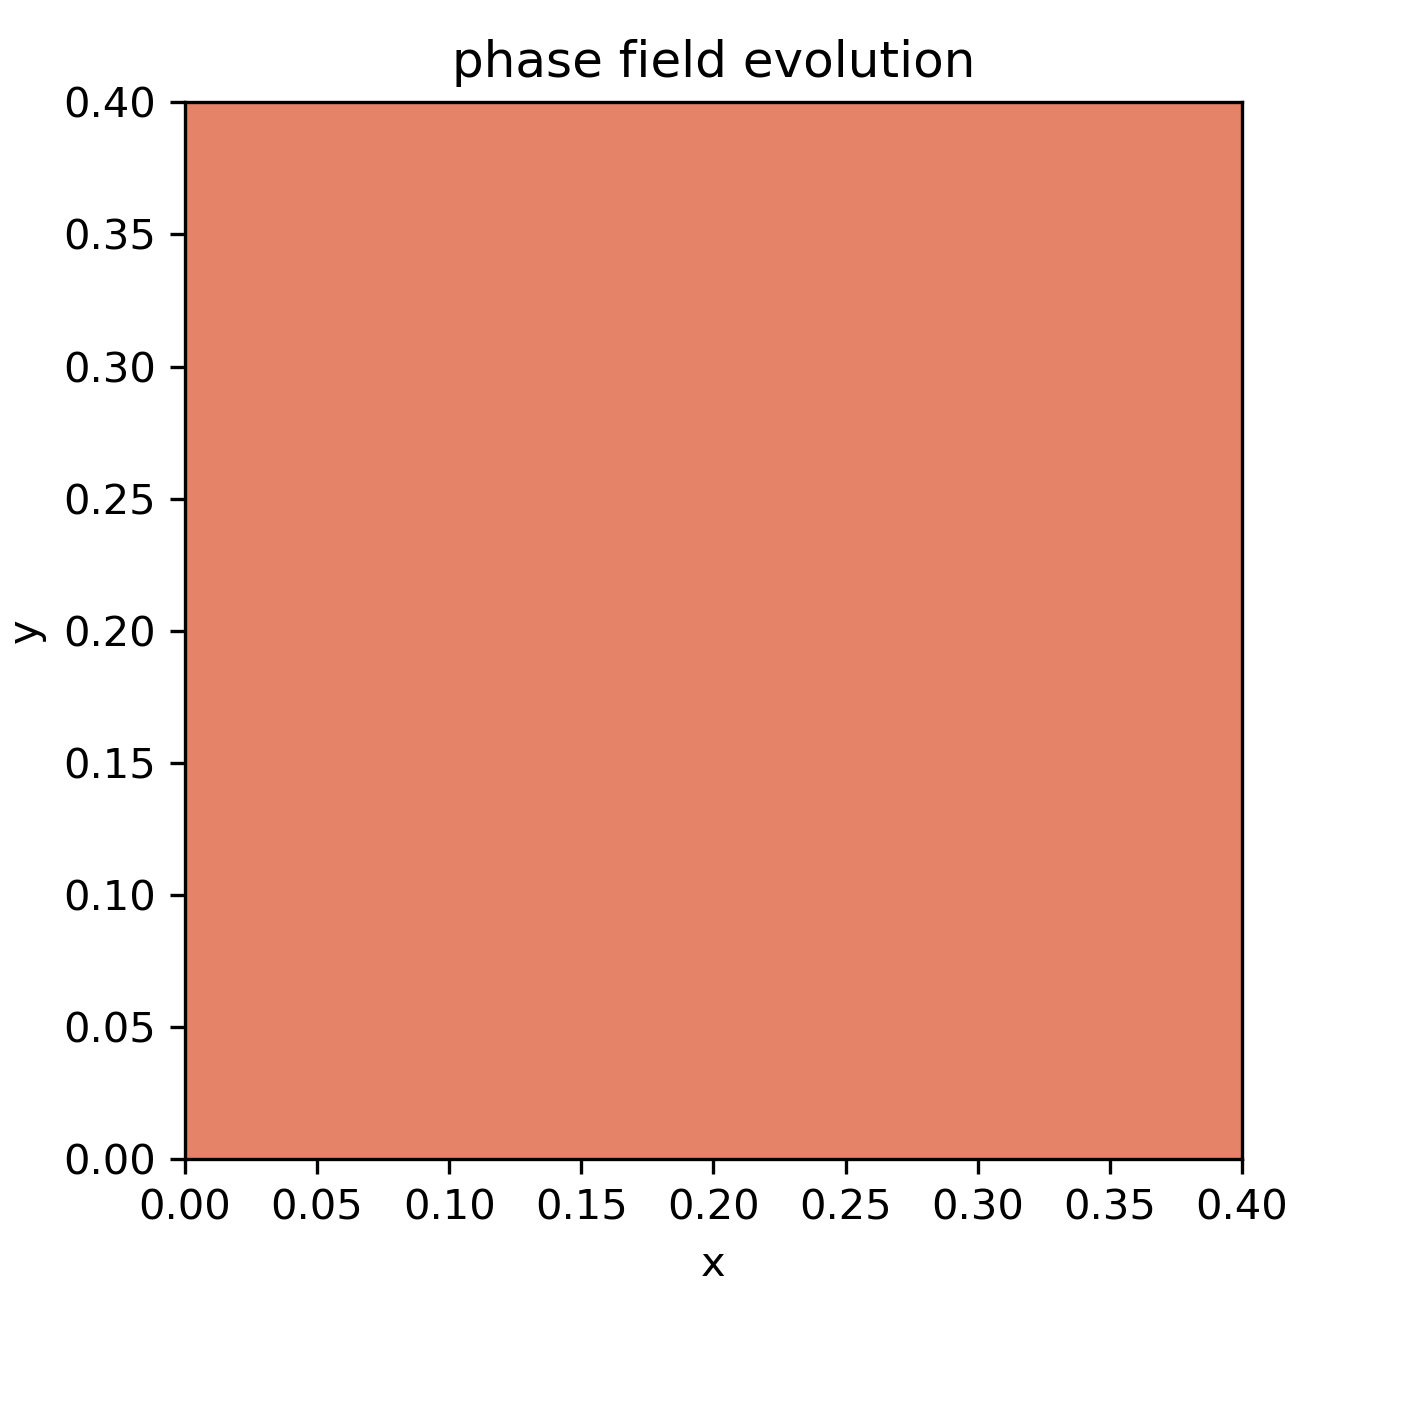}}    
      %\subfloat[t=0.25s]{\includegraphics[width=0.8\linewidth]{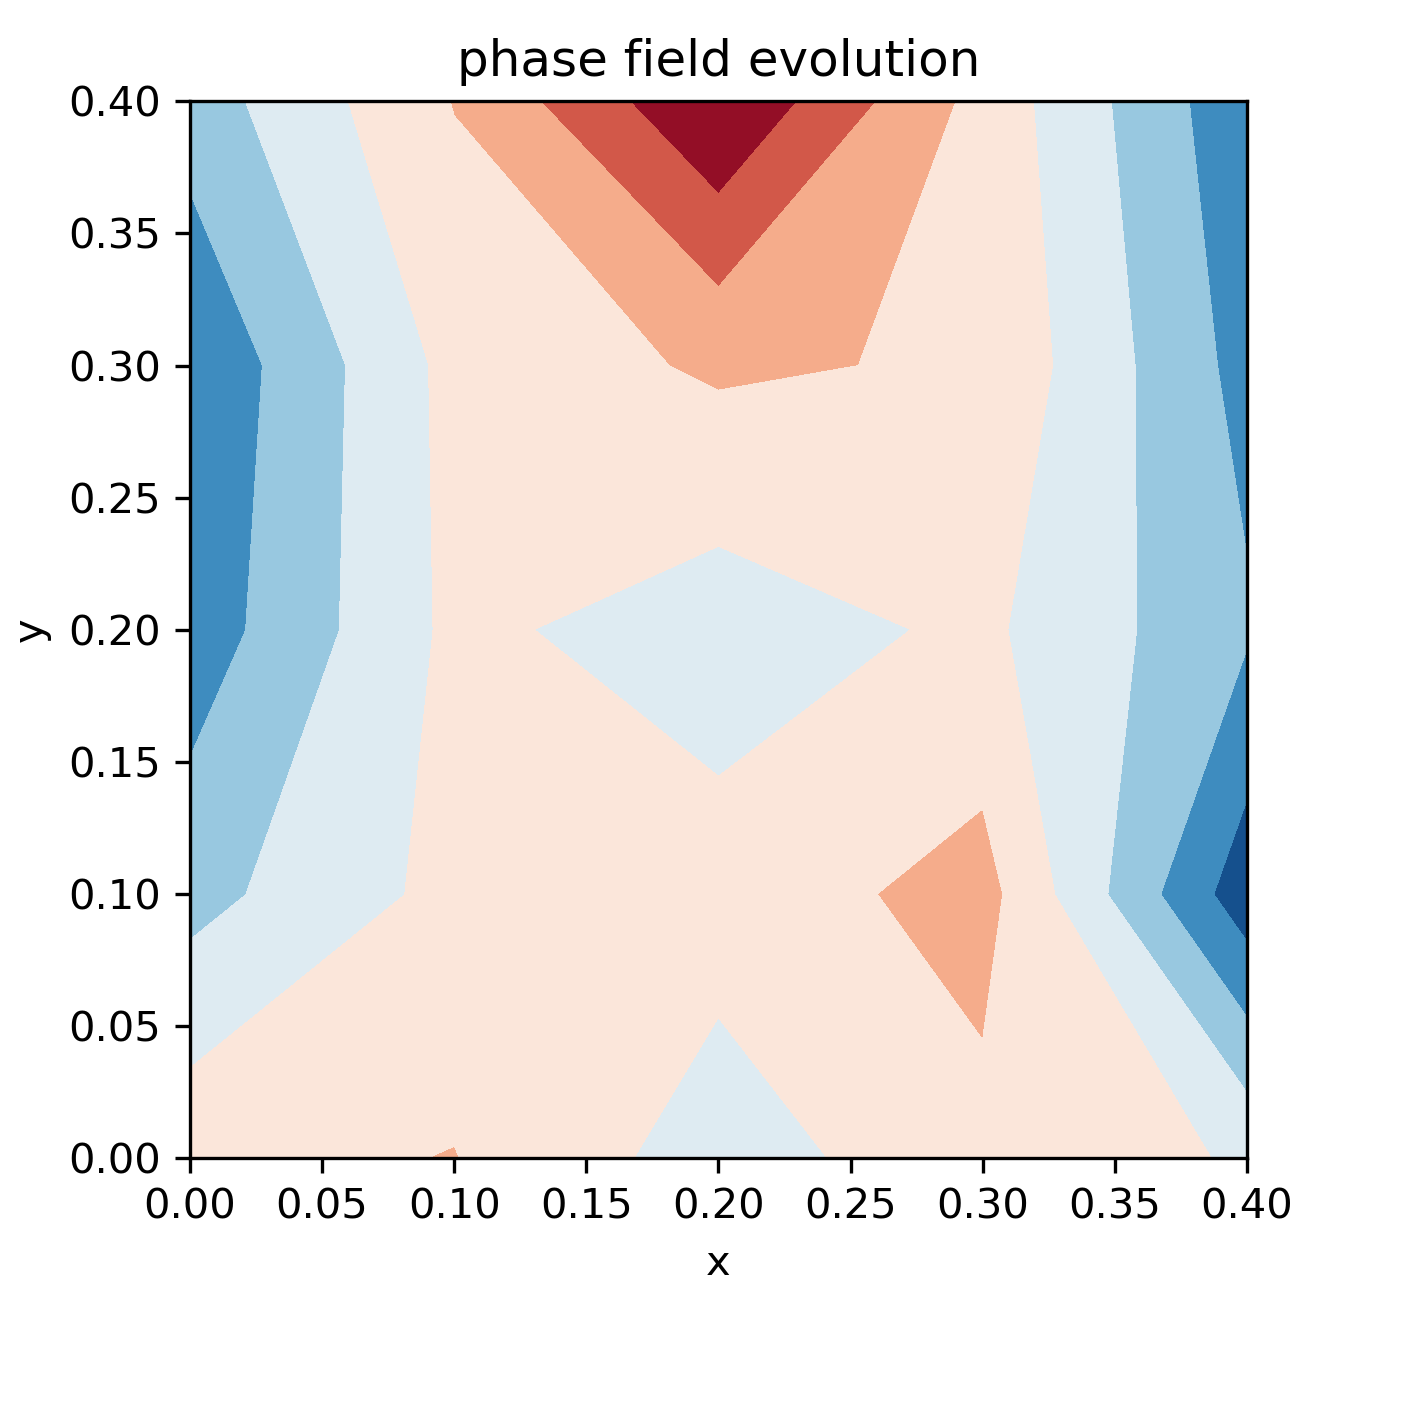}}
      \subfloat[t=0.50s]{\includegraphics[width=\linewidth]{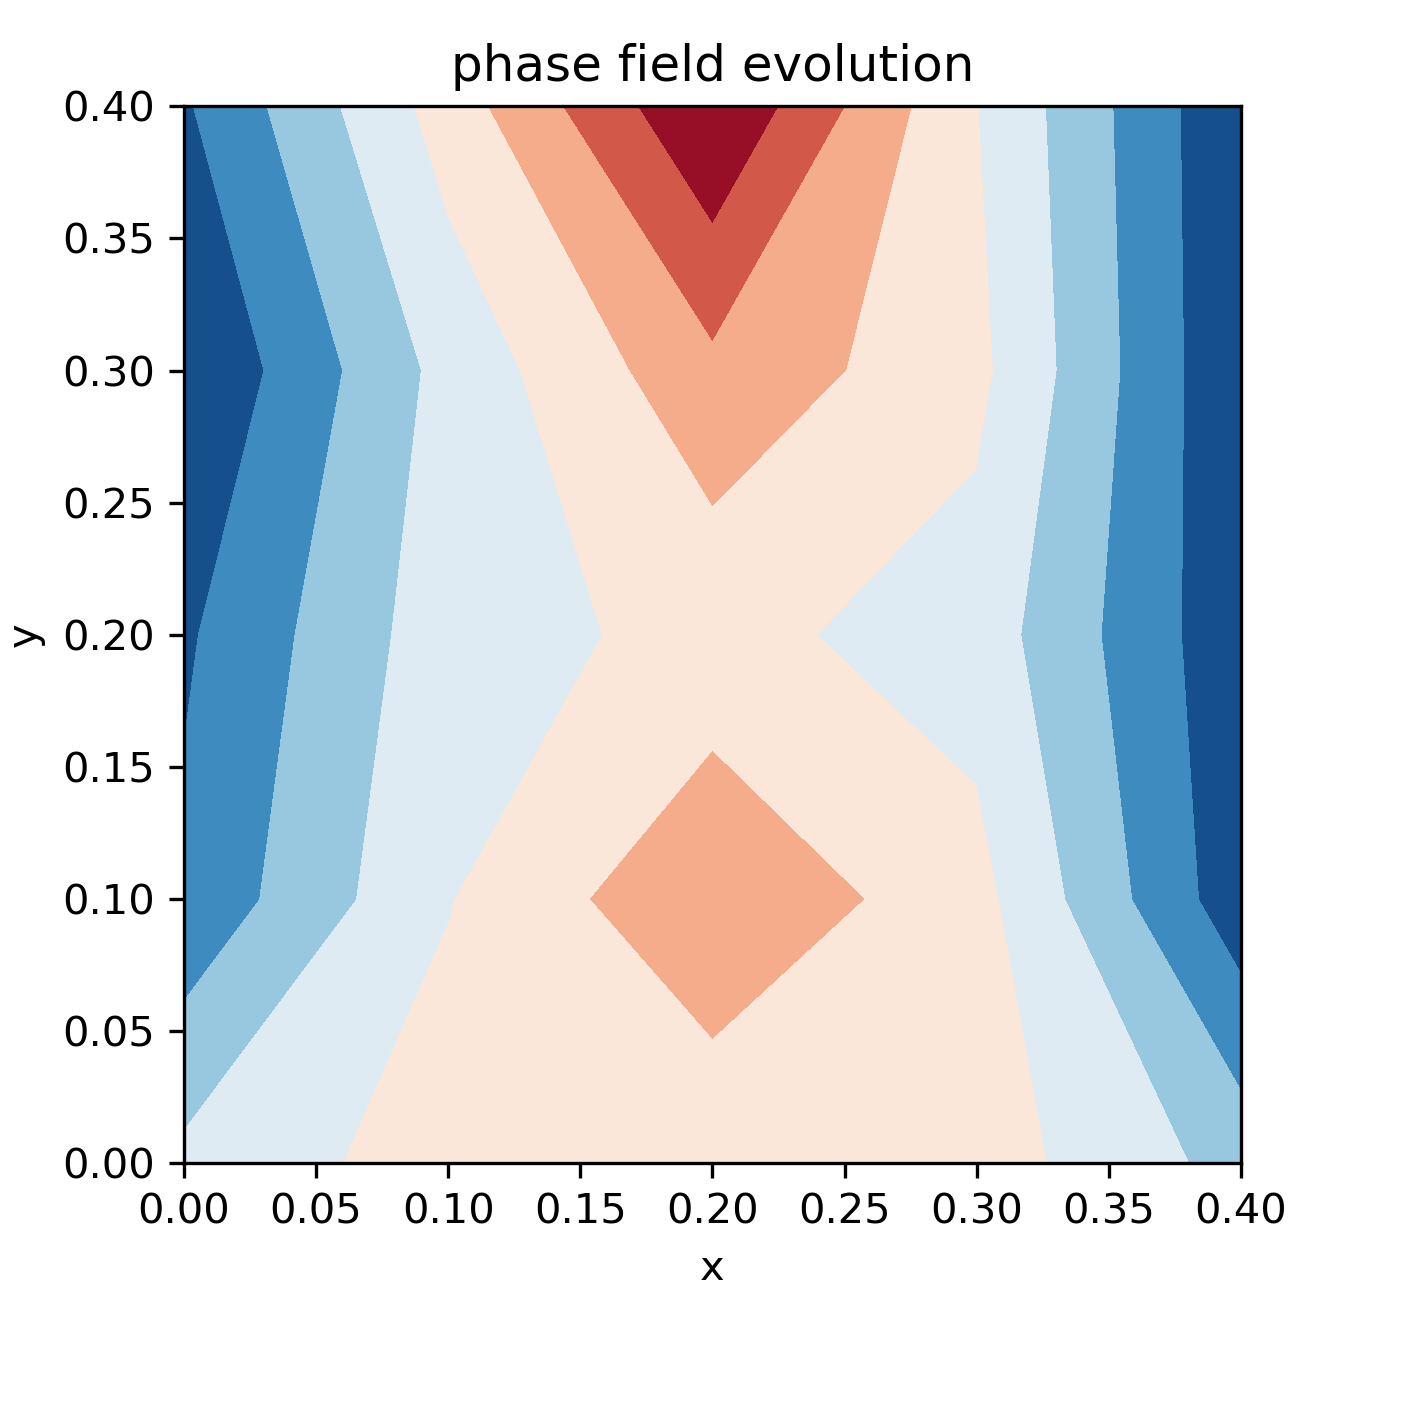}}
      %\subfloat[t=0.75s]{\includegraphics[width=0.8\linewidth]{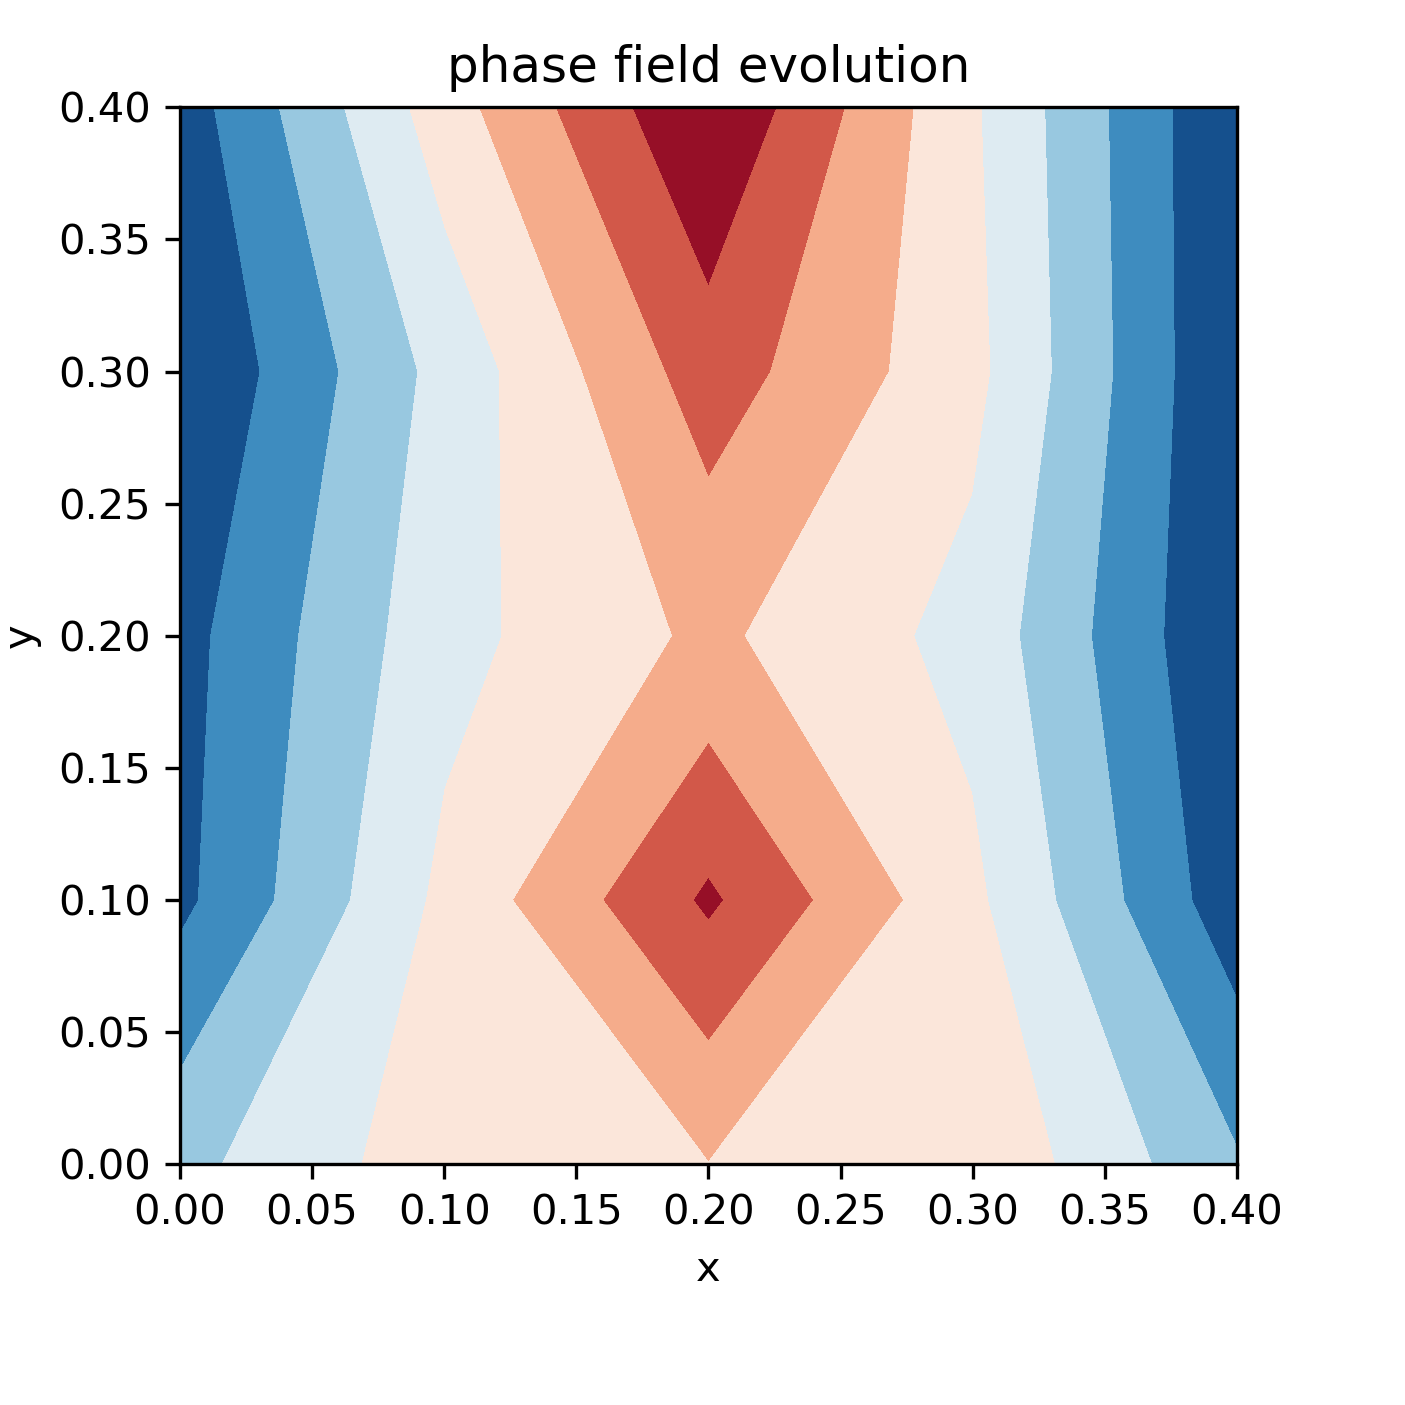}}
      \subfloat[t=1.00s]{\includegraphics[width=\linewidth]{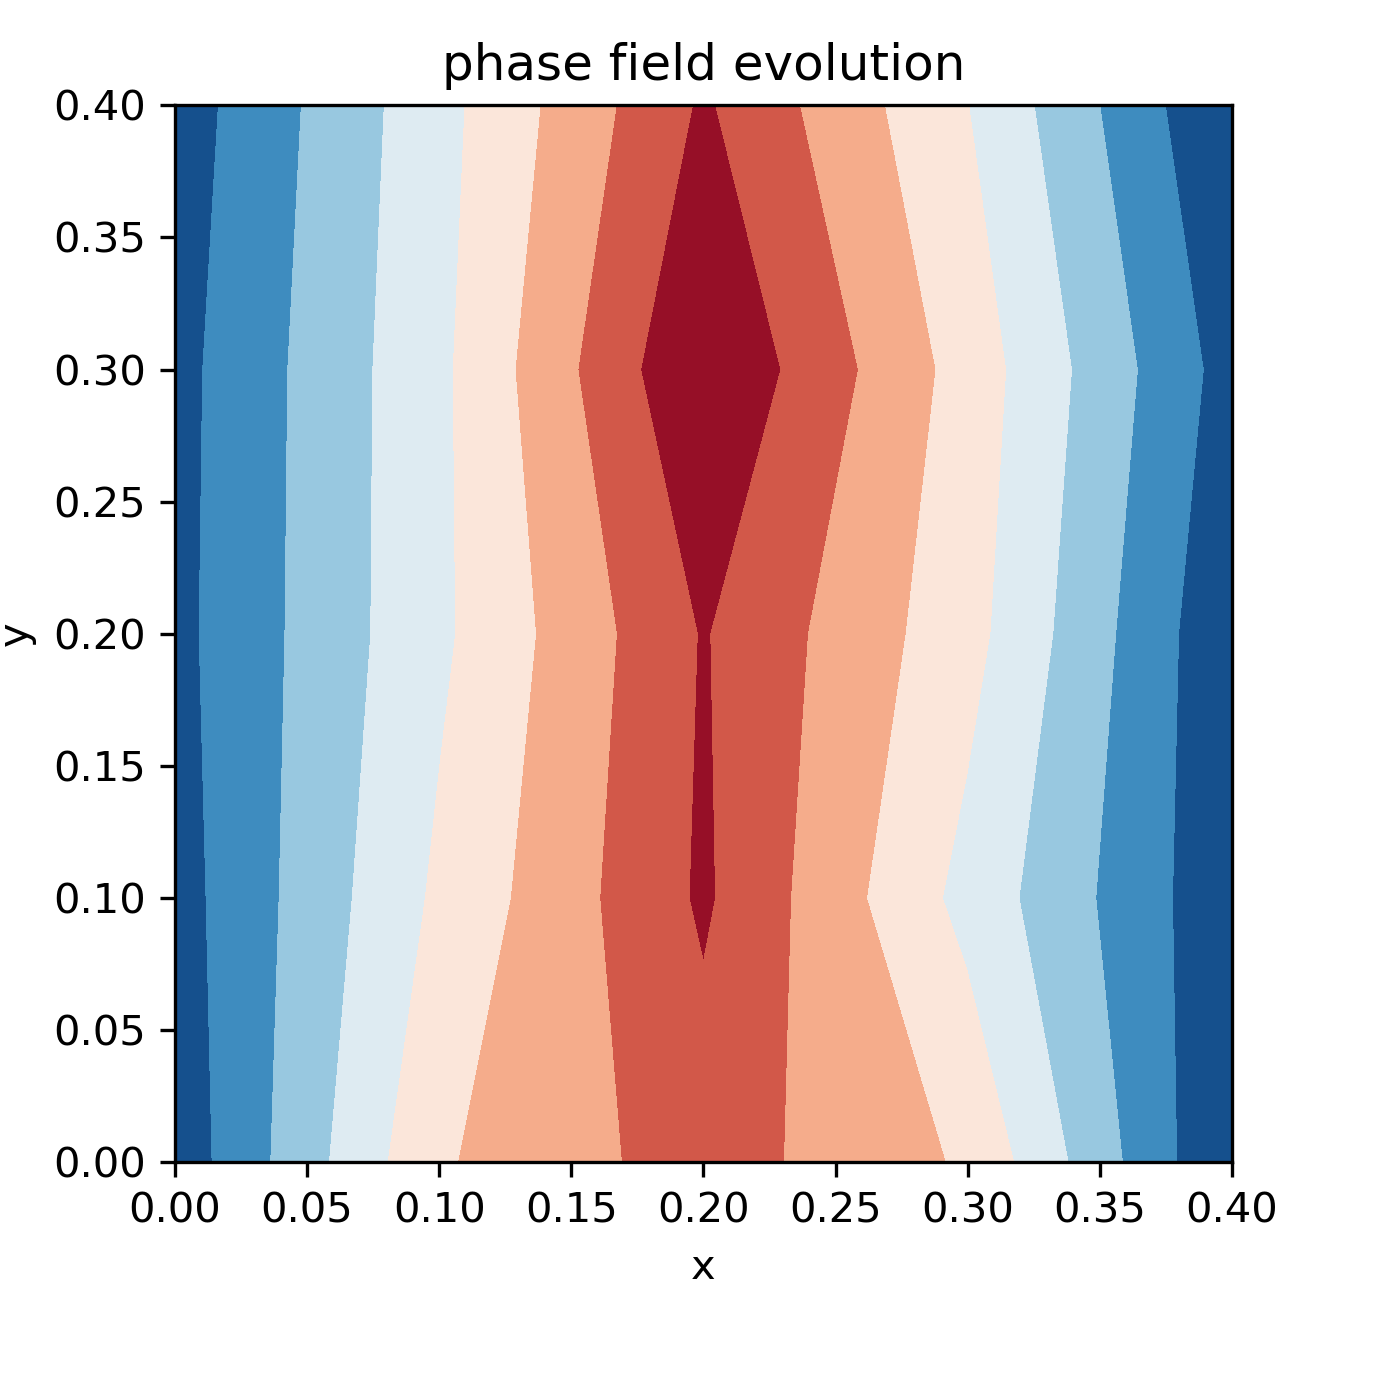}}
      %\subfloat[t=1.25s]{\includegraphics[width=0.8\linewidth]{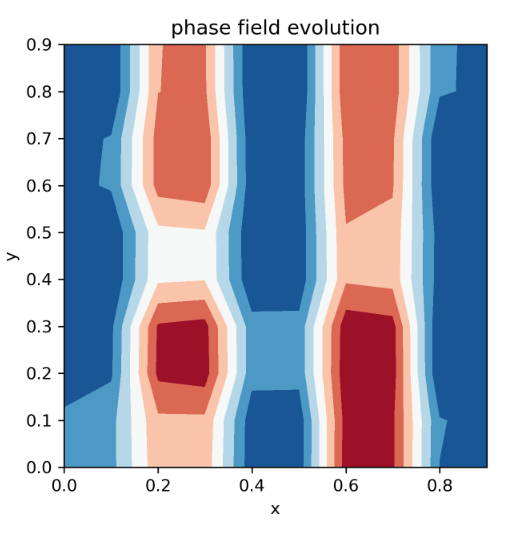}}\\
      
\end{multicols}

\begin{multicols}{3}
    % \hspace{3.2cm}
      \subfloat[Initial]{\includegraphics[width=\linewidth]{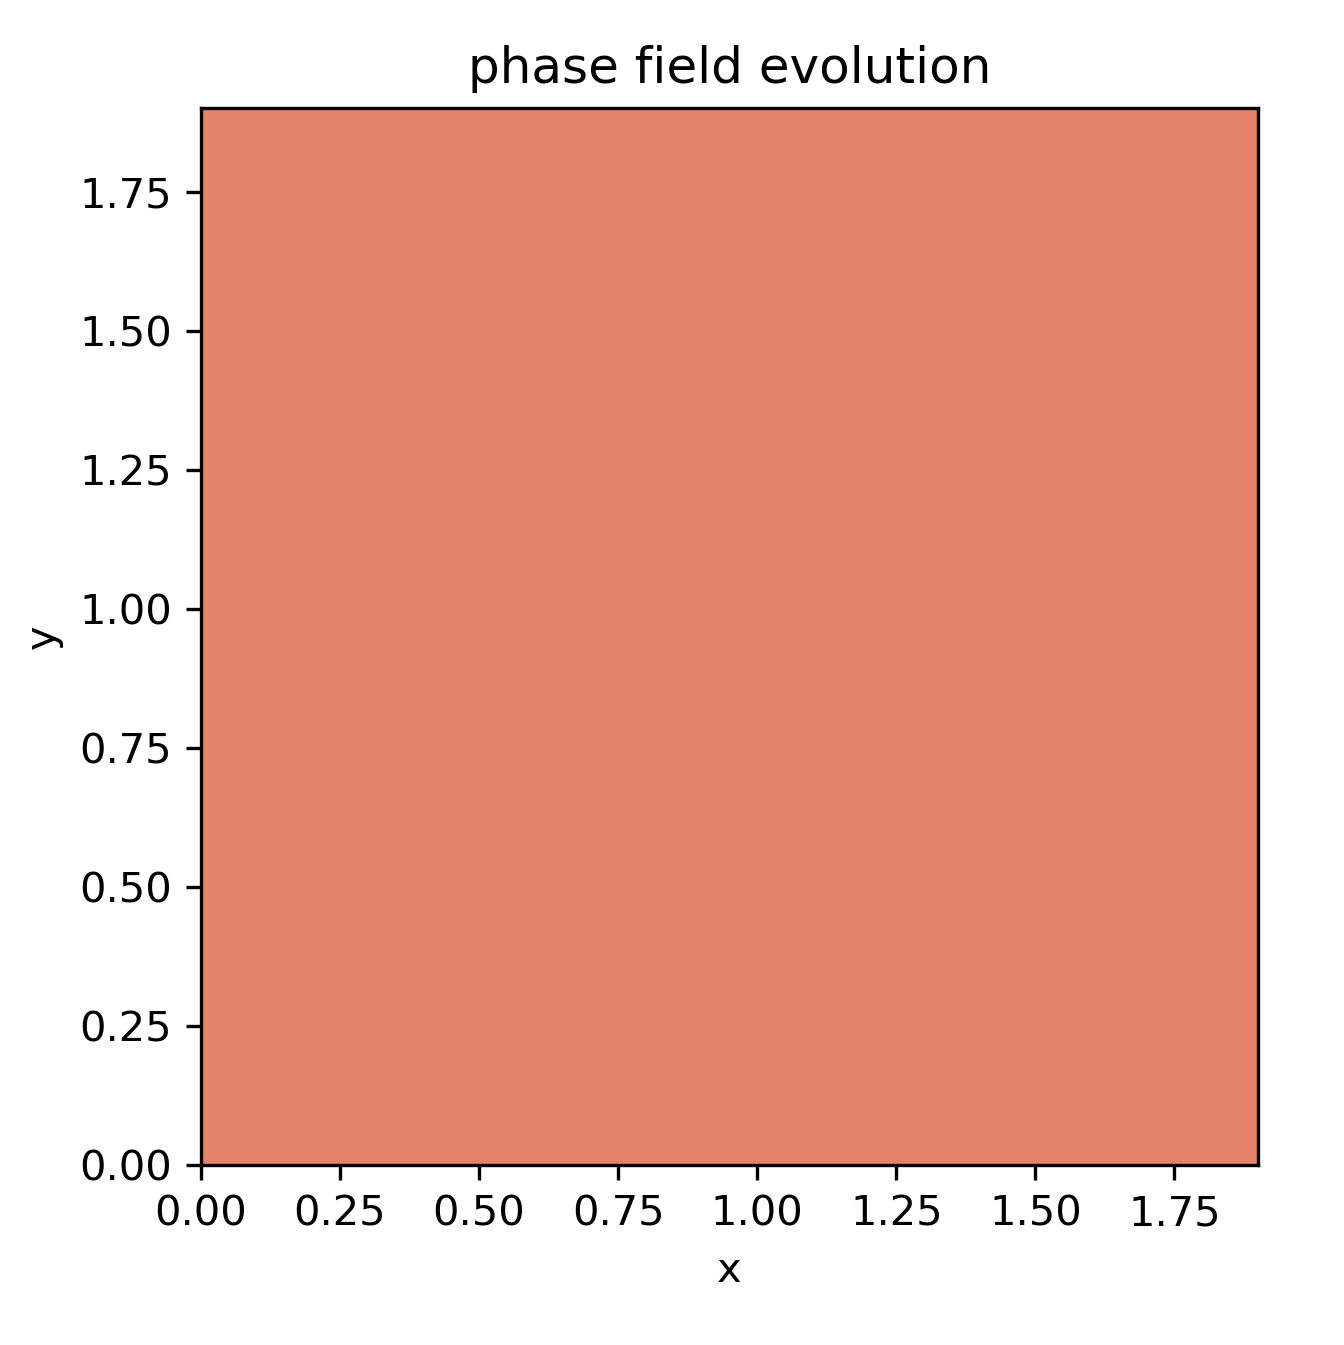}}    
      %\subfloat[t=0.25s]{\includegraphics[width=0.8\linewidth]{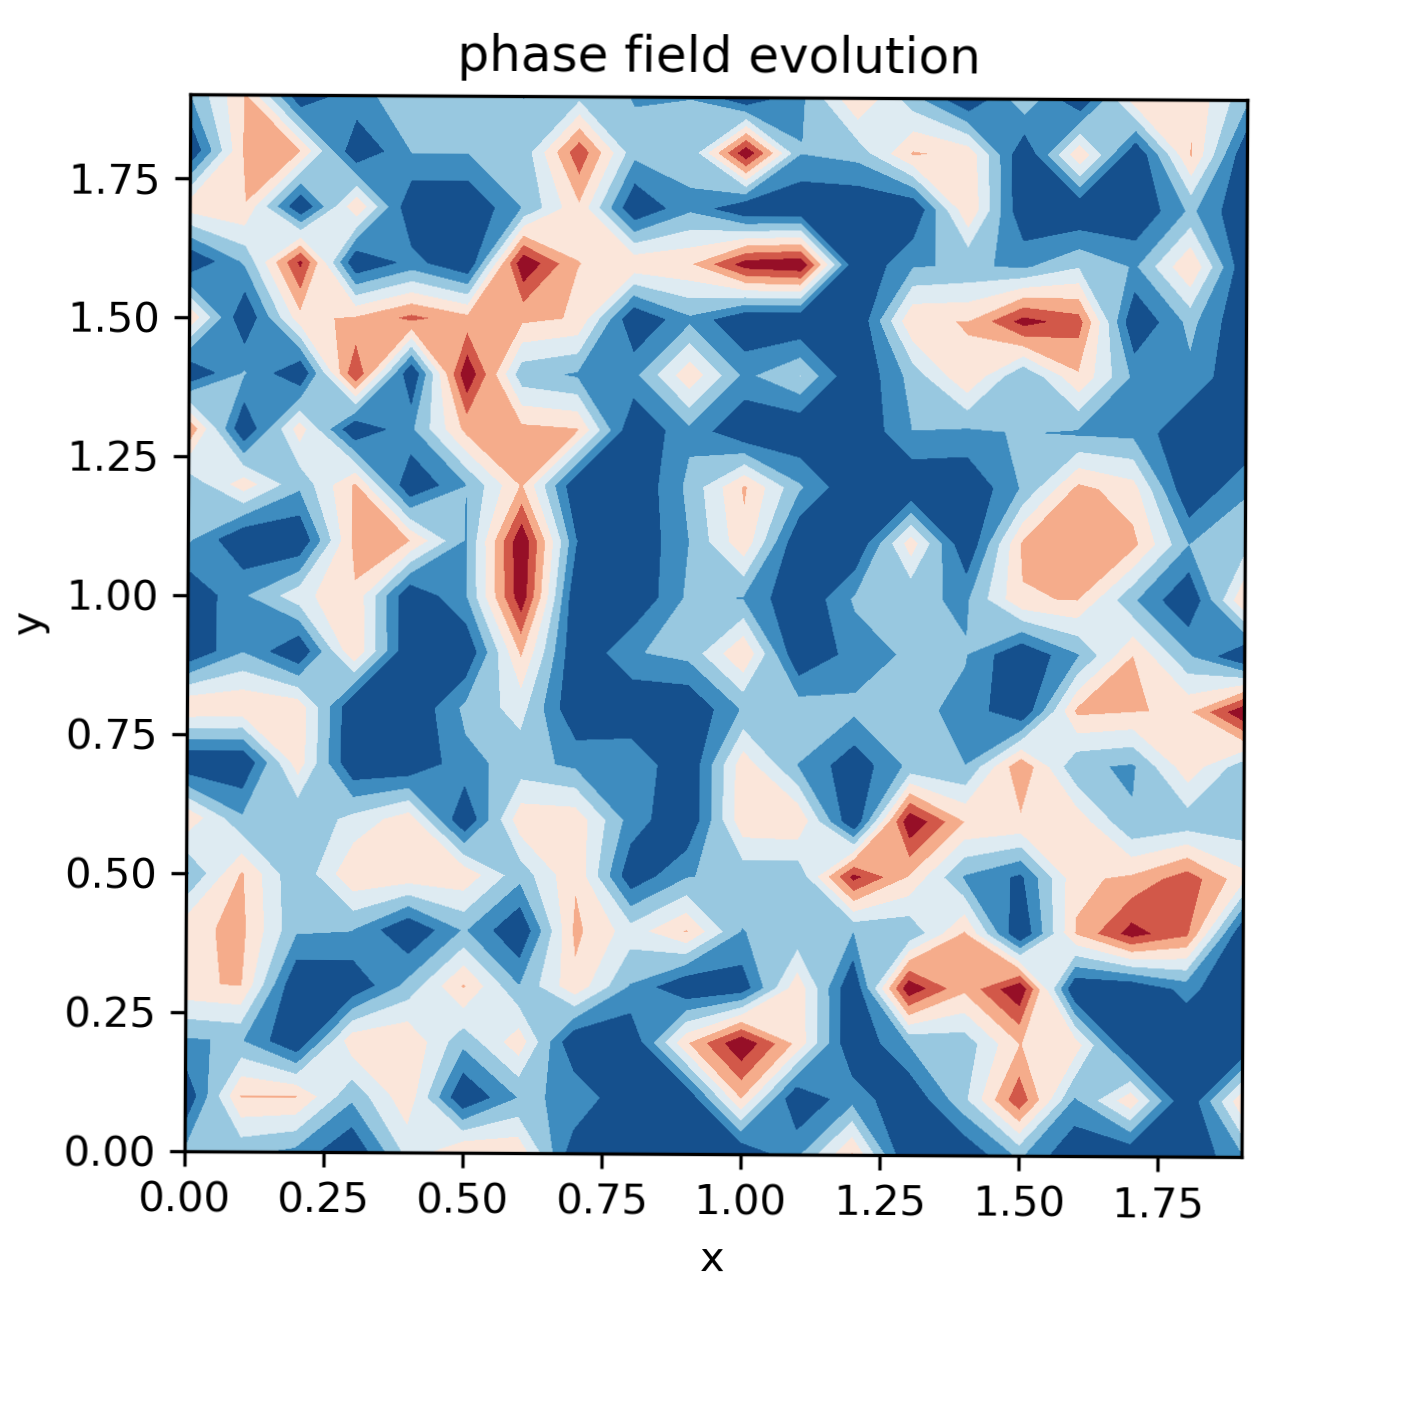}}
      \subfloat[t=0.50s]{\includegraphics[width=\linewidth]{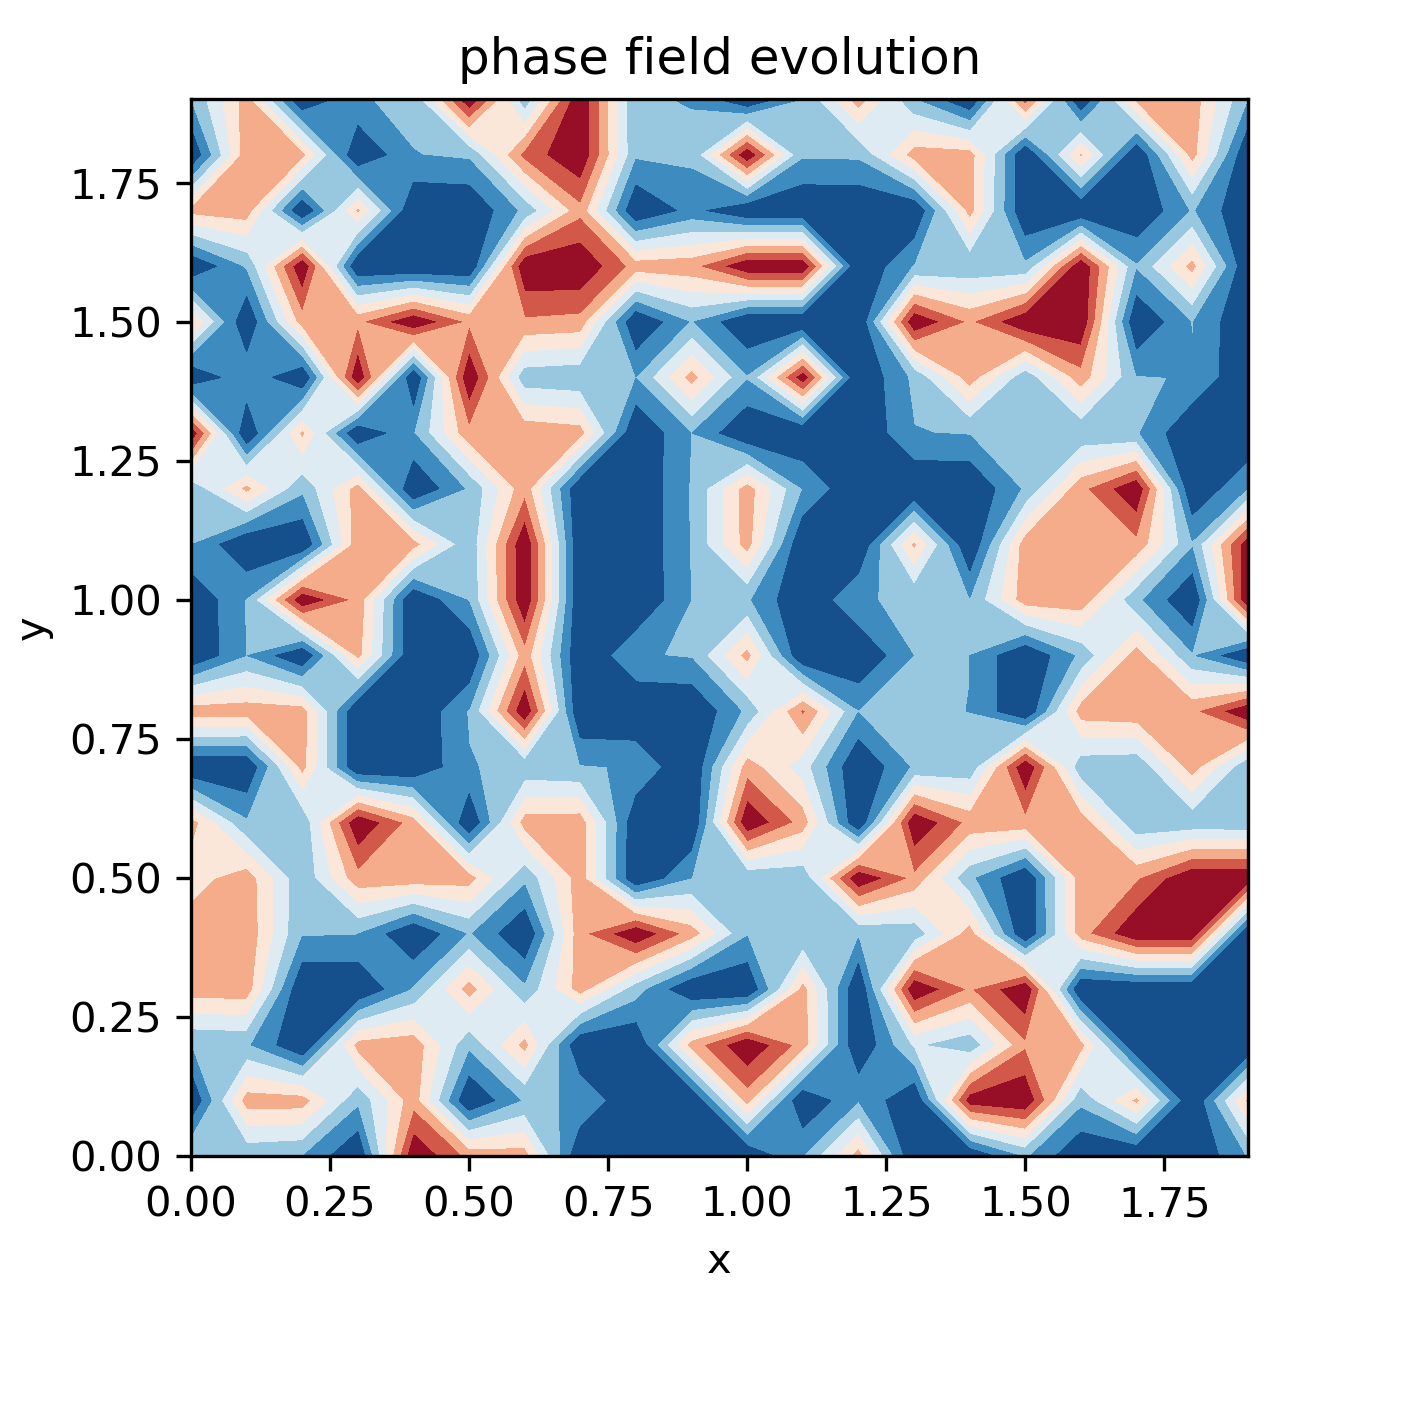}}
      %\subfloat[t=0.75s]{\includegraphics[width=0.8\linewidth]{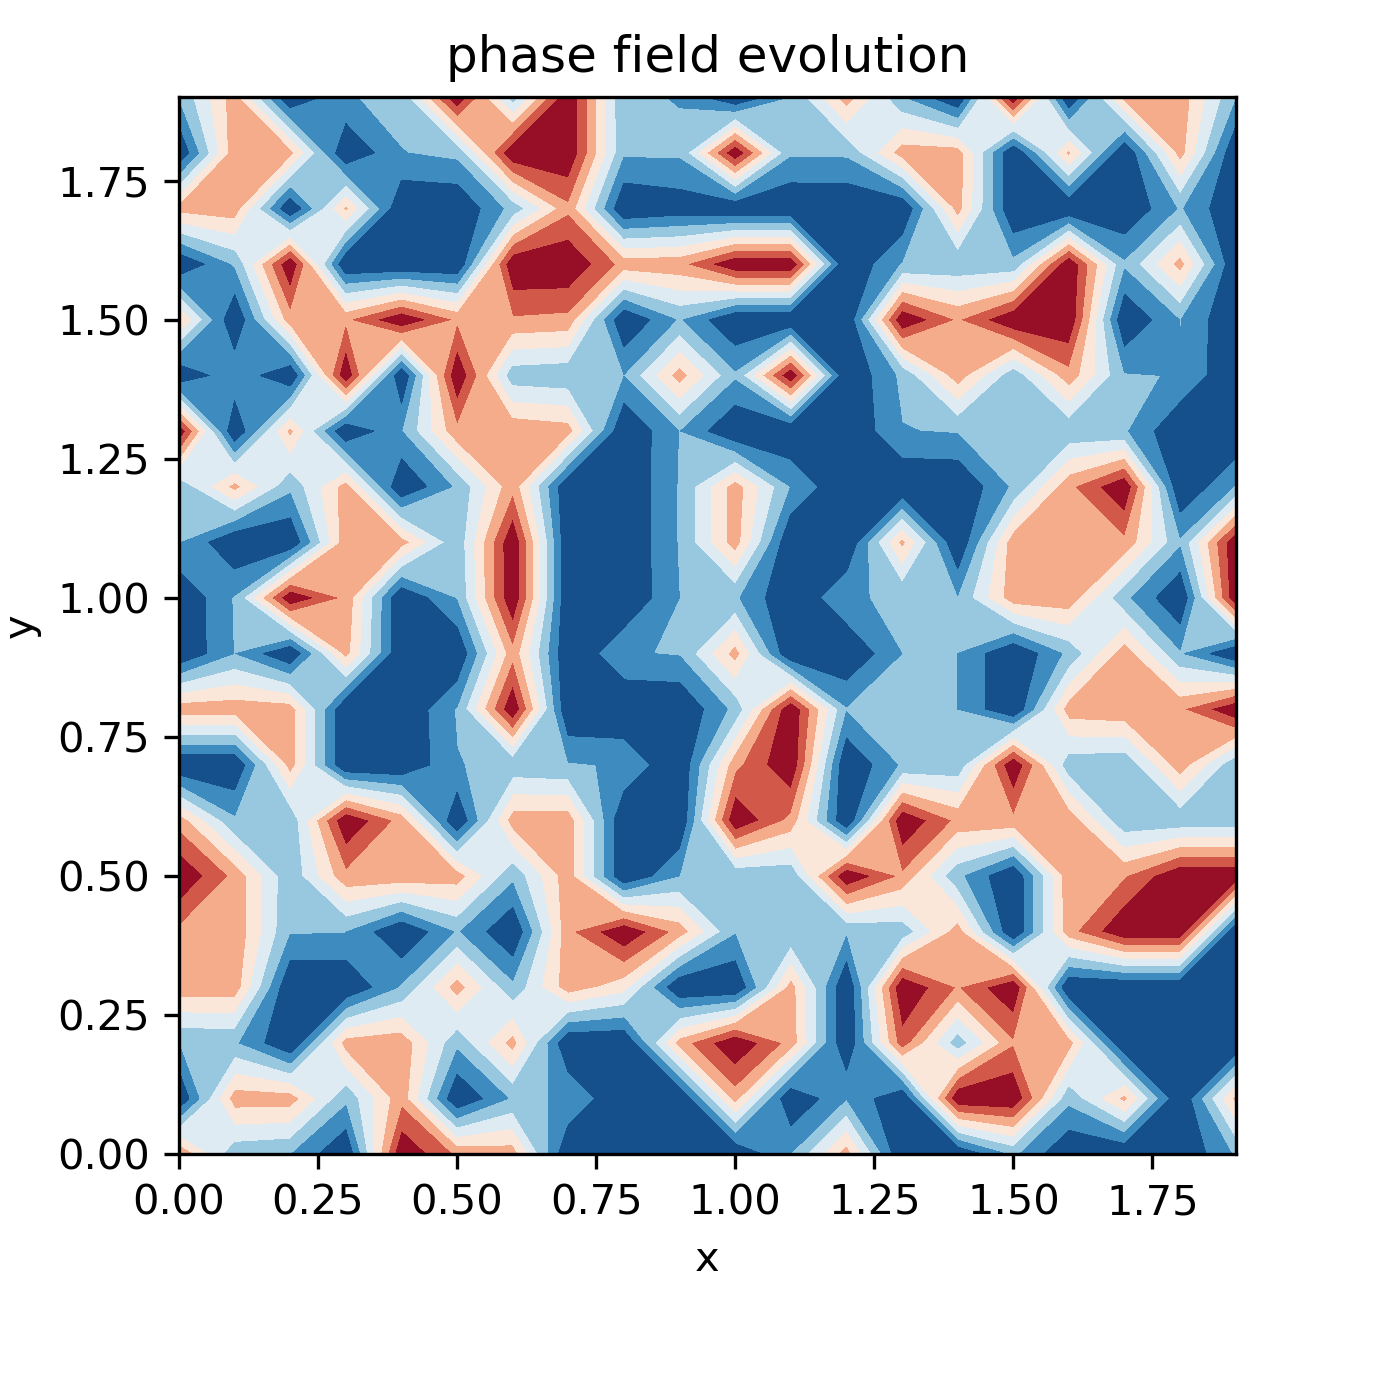}}
      \subfloat[t=1.00s]{\includegraphics[width=\linewidth]{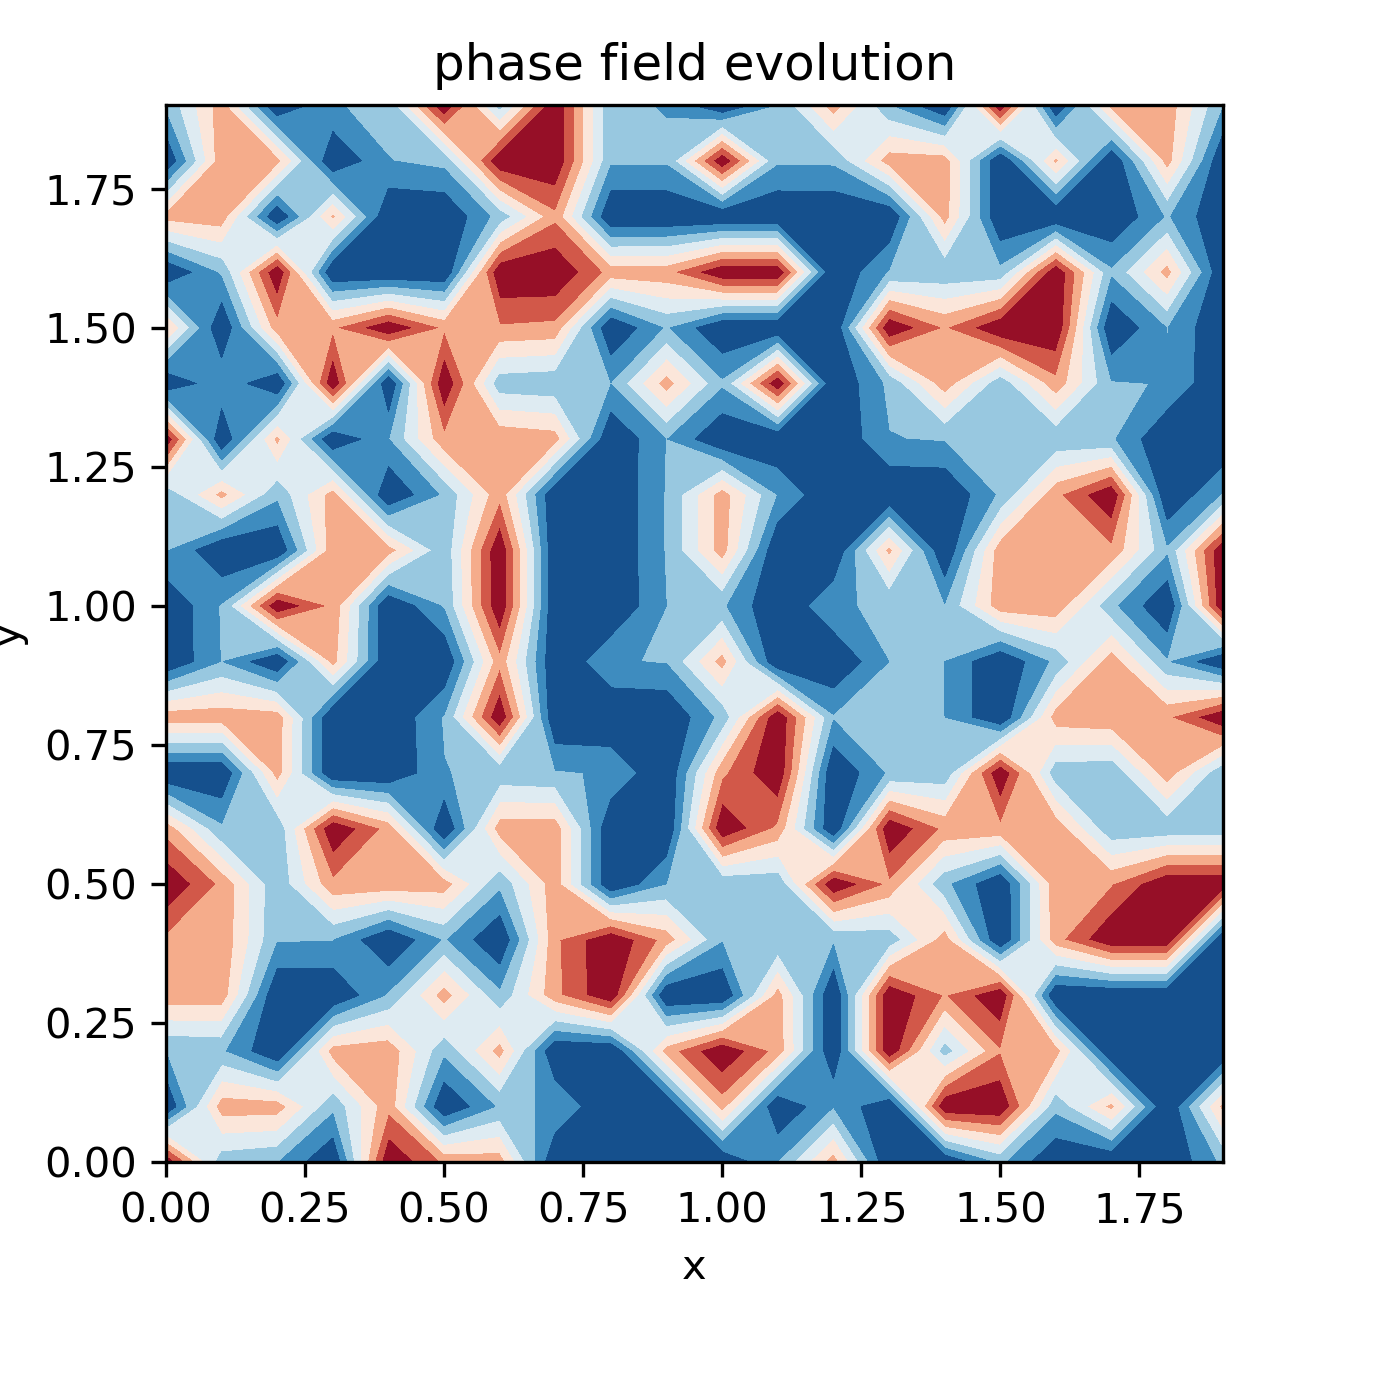}}
      %\subfloat[t=1.25s]{\includegraphics[width=0.8\linewidth]{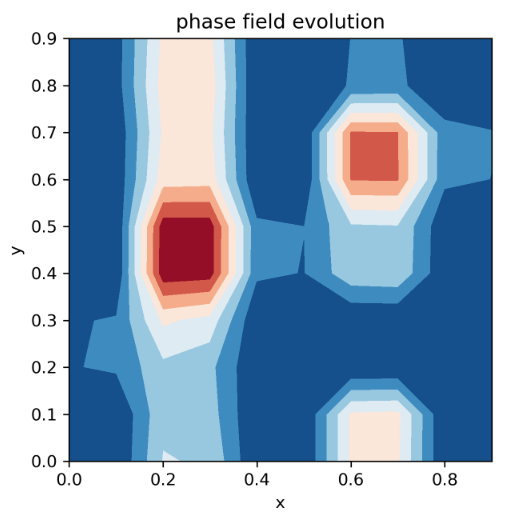}}\\

\end{multicols}
%\begin{multicols}{6}
%\captionsetup{width=.75\textwidth}
    \caption{{DDPG trajectories for a material model discretized as (a)$5 \times 5$, %(a)30\%U$_{MAX}$,
    (b)$20 \times 20$}} 
%\end{multicols}

\label{trajectory}
\end{figure}

%\input{Hybrid.tex}

% \subsection{Difference of Allen-Cahn and Cahn-Hilliard control}
% Determined by the different orders of derivatives of control variables ($T$ and $h$) in the evolution equations, the evolving behaviors of order parameter field from initial state to the desired goal state governed by Allen-Cahn and Cahn-Hilliard equations are completely distinct. For the Allen-Cahn equation, $T$ and $h$ are taken no derivative, and the value of order parameter can be therefore changed straightforwardly by choosing proper $T$ and $h$ (see $a_0-a_4$ in Fig. \ref{ACCH}). While for the Cahn-Hilliard equation, a Laplacian operation is applied to the term containing $T$ and $h$, which causes the order parameter field evolves to the desired state through the transport of order parameter field (see $b_0-b_4$ in Fig. \ref{ACCH}). Consequently, the demanded cost of controlling Allen-Cahn model to evolve from a given initial state to a goal state depends on the discrepancy of the initial state from the desired goal state, while that for Cahn-Hilliard model depends on the distribution of order parameter field as well.

% \begin{figure}
%     \centering
%     \includegraphics[width=1\linewidth]{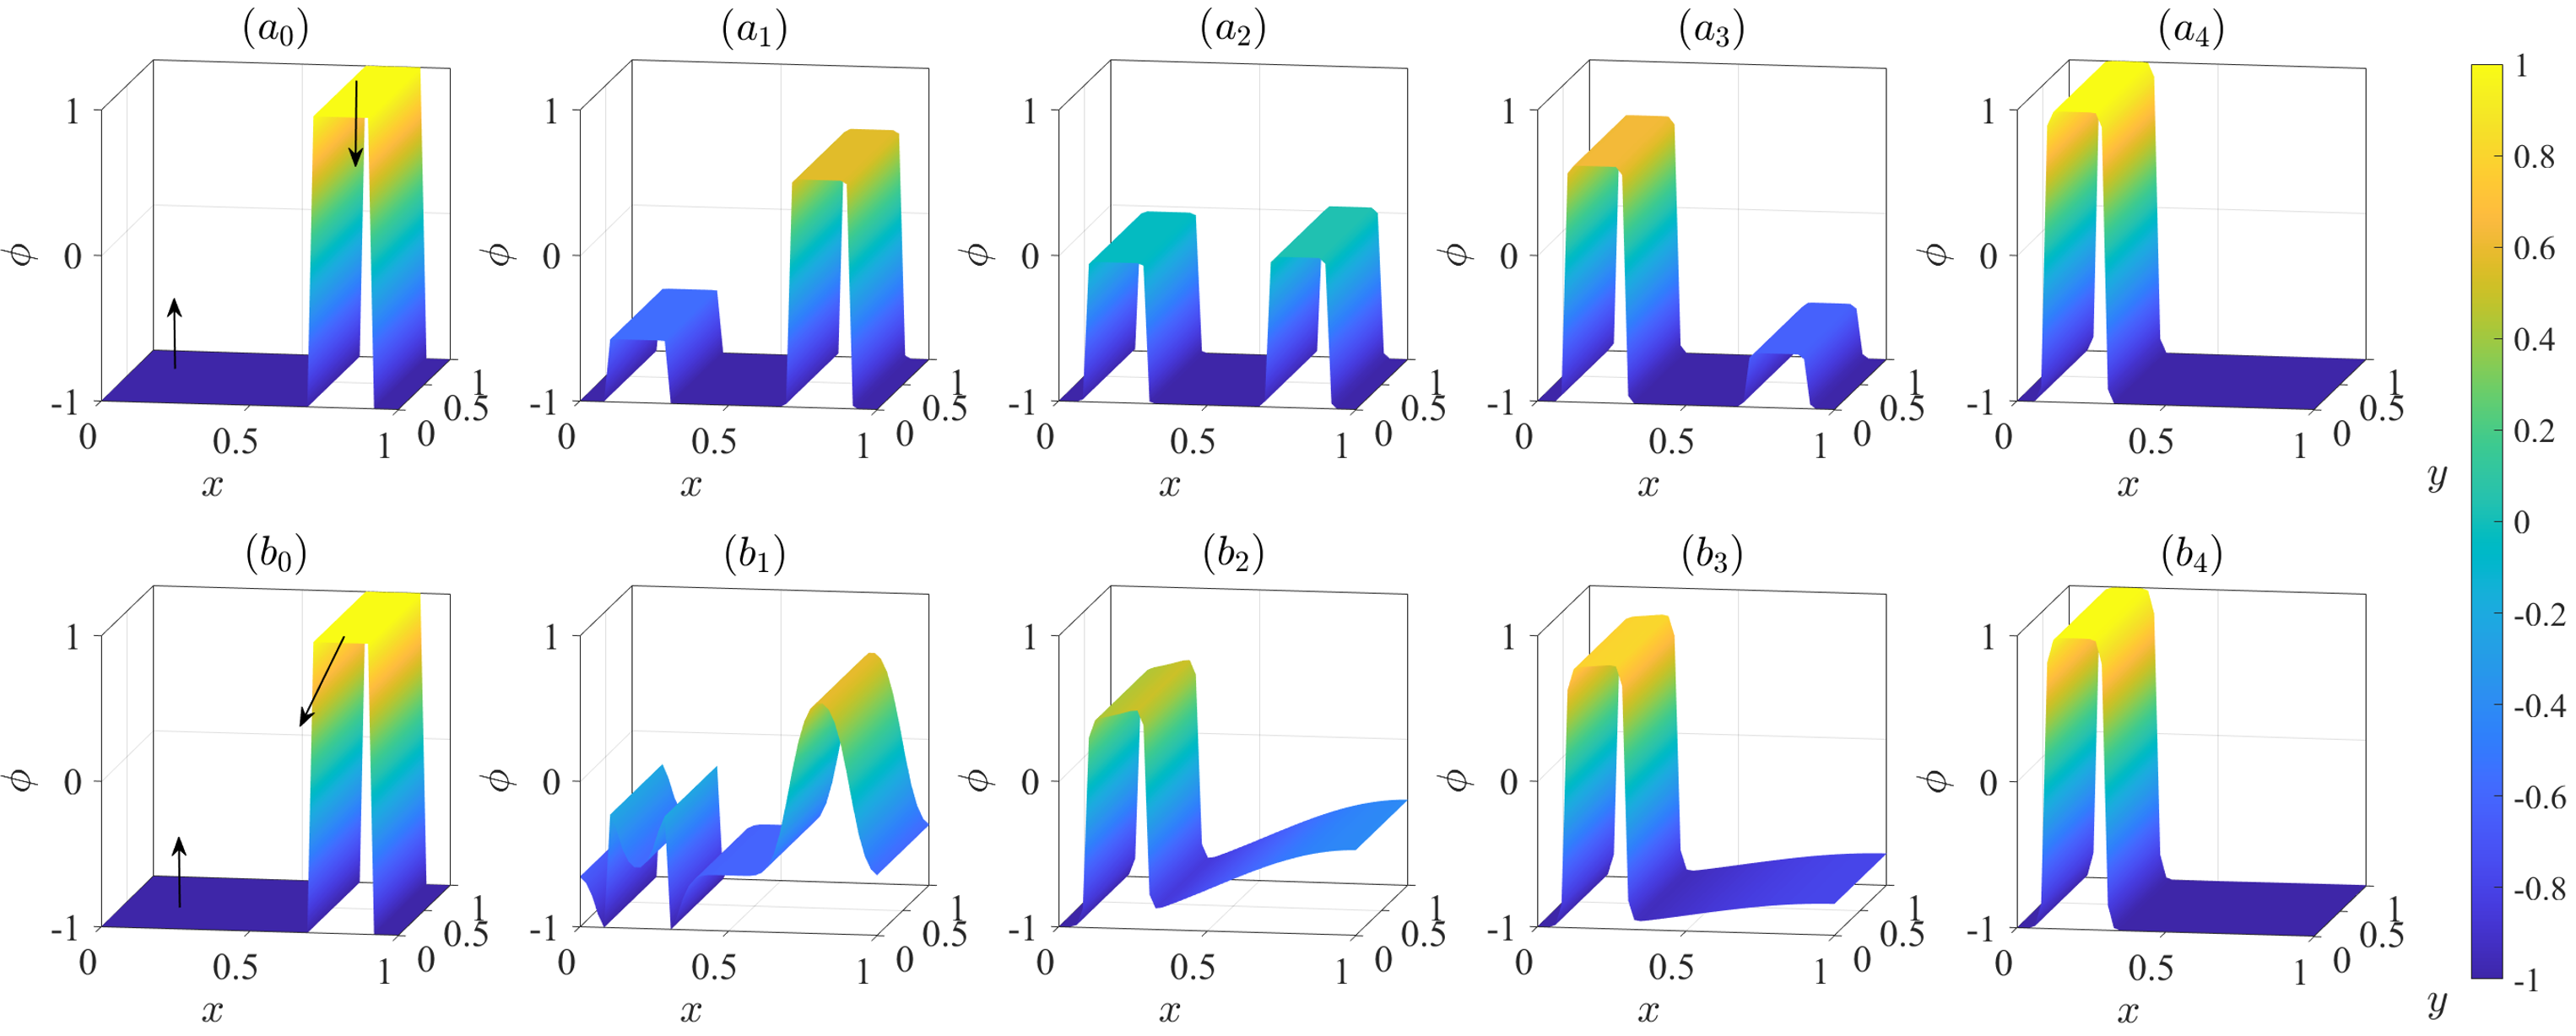}
%     \caption{Evolution process of order parameter field governed by Allen-Cahn ($a_0-a_4$) and Cahn-Hilliard ($b_0-b_4$) equations. $a_0$ and $b_0$ represent the initial states that be controlled to evolve to the final states represented by $a_4$ and $b_4$, respectively.}
%     \label{ACCH}
% \end{figure}
